# Supplementary material for: "What is the value of {templates}?" Rethinking Document Information Extraction Datasets for LLMs
Source: arXiv:2410.15484 source file (2024-10-20)
Supplement: Supplementary file 1 [file a0pastdatasets.tex]

% Not sure if this is needed in the appendix or main paper

\section{Past datasets and drawbacks}
\begin{itemize}
    \item FLAN \citep{wei-22-finetuned}: Dataset for general NLP tasks. Each task/dataset gets 10 templates to fill for diversity. Furthermore, each task/dataset has up to three additional templates that ask for generation. No task regarding information extraction so no direct comparison to how questions exactly from the text are given (closest is reading comprehension).
    \item Flan-PALM \citep{chung-22-scaling}: Similar to FLAN but encorporates additional datasets
    \item InstructGPT \citep{ouyang-22-training}: Not really relevant, did not convert any datasets
    \item Self-Instruct \citep{wang-23-self}: Again not really converting datasets
    \item LlamaV2 \citep{touvron-23-llama}: Used dialogue datasets
    \item mPlug-DocOwl \citep{ye-23-mplug}: DocAI Dataset. For Information extract, questions are created used a single template with no alternatives. Very not diverse
    \item UDOP \citep{tang-23-unifying}: Like mPlug-DocOwl, only uses one  template
    \item DUDE benchmark \citep{landeghem-23-document}: General new VQA dataset
    \item 
\end{itemize}

\section{Other Relevant Work}
\begin{itemize}
    \item \citet{hegde-23-analyzing}
\end{itemize}
